# Supplementary material for: Iteratively Learning Representations for Unseen Entities with Inter-Rule Correlations
Source: arXiv:2305.10531 source file (2023-09-04)
Supplement: Supplementary file 1 [file appendix.tex]

\appendix
% \section{Appendix}

\section{Appendix}
